# Supplementary material for: Robustly representing uncertainty in deep neural networks through sampling
Source: arXiv:1611.01639 source file (2018-01-20)
Supplement: Supplementary file 1 [file supplement.pdf]

# Supplementary Material: Robustly representing uncertainty through sampling in deep neural networks

**Patrick McClure**
MRC Cognition and Brain Sciences Unit
University of Cambridge
patrick.mcclure@mrc-cbu.cam.ac.uk

**Nikolaus Kriegeskorte**
Department of Psychology
Columbia University
nk2765@columbia.edu

## 1 Methods

### 1.1 L2 regularization and the KLD between Gaussians

The Kullback–Leibler divergence (KLD) between $\mathcal{N}(\mu_q, \sigma_q^2)$ and $\mathcal{N}(\mu_p, \sigma_p^2)$ can be calculated using:

$$KL(q(w_{i,j})||p(w_{i,j})) = \frac{(\mu_q - \mu_p)^2}{2\sigma_p^2} + \log\frac{\sigma_p}{\sigma_q} + \frac{\sigma_q^2}{2\sigma_p^2} - \frac{1}{2} \tag{1}$$

In the case where $\mathcal{N}(\mu_p, \sigma_p^2)$ is a pre-defined prior and $\sigma_q$ is not a function of the learnable parameters $V$:

$$\underset{V}{\operatorname{argmin}}\, KL(q(w_{i,j})||p(w_{i,j})) = \underset{V}{\operatorname{argmin}}\, \frac{(\mu_q - \mu_p)^2}{2\sigma_p^2} \tag{2}$$

For $\mu_p = 0$, this is equivalent to L2 regularization where the L2-coefficent is equal to $1/\sigma_p^2$. However, in the case where $\sigma_q$ is a function of $V$, such as for Gaussian dropout/dropconnect, this equivalence does not hold. In [5], Kingma et al. used a log-uniform prior instead of a Gaussian prior in order to bypass this and make the KLD not a function of $V$. In our derivations, we minimize a lower bound of Equation 1 constructed using the fact that the sum of the terms that include $\sigma_q$ and the constant term is greater than or equal to 0:

$$KL(q(w_{i,j})||p(w_{i,j})) \geq \frac{(\mu_q - \mu_p)^2}{2\sigma_p^2} \tag{3}$$

Note that a similar lower bound can be derived for the KLD between two multivariate Gaussians.

### 1.2 Gaussian "reparameterization trick"

As discussed in [5], for a matrix $W$ of Gaussian random variables can be sampled using the "reparamaterization trick":

$$w_{i,j} \sim \mathcal{N}(\mu_{v_{i,j}}, \alpha v_{i,j}^2) \tag{4}$$

$$w_{i,j} = f(v_{i,j}, \epsilon_{i,j}) = v_{i,j} + \sqrt{\alpha} v_{i,j} \epsilon_{i,j} \tag{5}$$

Second workshop on Bayesian Deep Learning (NIPS 2017), Long Beach, CA, USA.

where $\epsilon_{i,j} \sim \mathcal{N}(0,1)$, $\alpha = p/(1-p)$, and $p$ is the dropout or dropconnect drop probability. Given a deterministic, differentiable, and monotonic mapping $W = f(V,\epsilon)$, $q_V(W)dW = p(\epsilon)d\epsilon$. As a result:

$$\int q_V(W)l(W)dW = \int p(\epsilon)l(W)d\epsilon = \int p(\epsilon)l(f(V,\epsilon))d\epsilon \tag{6}$$

### 1.3 MC Gaussian Dropconnect and Dropout

For approximate inference, variational distribution $q_V(W)$ is learned by maximizing the log-evidence lower bound over parameters $V$ [1; 2; 3; 4]:

$$\log(p(D_{train})) \geq \int \log p(D_{train}|W)q_V(W)dW - KL(q_V(W)||p(W)) \tag{7}$$

For either Gaussian dropout or dropconnect, each element of $W$ is sampled from a Gaussian distribution, $\mathcal{N}(v_{i,j}, \sigma^2_{v_{i,j}})$, where $\sigma^2_{v_{i,j}} = \alpha\mu^2_{v_{i,j}}$. $W$ can then be sampled using the Gaussian "reparameterization trick", which allows Equation 7 to be rewritten as:

$$\log(p(D_{train})) \geq \int_\epsilon \log p(D_{train}|W)q(\epsilon)d\epsilon - KL(q_V(W)||p(W)) \tag{8}$$

where $\epsilon$ is a vector containing each $\epsilon_{i,j}$.

This results in the following minimization objective function:

$$\mathcal{L}_V := -\int_\epsilon \log(p(D_{train}|W))q(\epsilon)d\epsilon + KL(q_V(W)||p(W) \tag{9}$$

By using L2 regularization, we are optimizing a lower-bound of the KLD between $q_V(W)$ and the prior $p(w_{i,j}) = \mathcal{N}(0, \lambda^{-1})$ as previously shown:

$$\mathcal{L}_V \geq \widetilde{\mathcal{L}}_V := -\int_\epsilon \log(p(D_{train}|W))q(\epsilon)d\epsilon + \frac{\lambda}{2}\mathbf{v}\mathbf{v}^\intercal \tag{10}$$

where $\mathbf{v}$ is a vector containing each $v_{i,j}$ and $\epsilon$ is a vector containing each $\epsilon_{i,j}$.

Approximating using Monte Carlo integration for training (Eq. 11) and testing (Eq. 12):

$$\widetilde{\mathcal{L}}_\mathbf{v} :\approx -\frac{1}{n}\sum_\epsilon \log(p(D_{train}|W)) + \frac{\lambda}{2}\mathbf{v}\mathbf{v}^\intercal \tag{11}$$

$$p(D_{test}) \approx \frac{1}{n}\sum_\epsilon p(D_{test}|W) \tag{12}$$

where $\epsilon_{i,j} \sim \mathcal{N}(0,1)$ for Gaussian dropconnect and $\epsilon_{i,*} \sim \mathcal{N}(0,1)$ for Gaussian dropout.

### 1.4 MC spike-and-slab Dropout

For MC spike-and-slab dropout, the weight matrix $W = B \circ G$ where $b_{i,*} \sim Bern(1-p_{do})$ and $g_{i,j} \sim \mathcal{N}(v_{i,j}, \sigma^2_{v_{i,j}})$, similar to the method discussed in [6]. Instead of directly performing variational inference for $p(W|D_{train})$, we find a variational distribution, $q_V(B,G)$ for $p(B,G|D_{train})$ using:

$$\begin{aligned} log(p(D_{train})) \geq &\sum_B \int_G \log(p(D_{train}|B,G))q_V(B,G)dG \\ &- KL(q_V(B,G)||p(B,G)) \end{aligned} \tag{13}$$

Assuming independence between the random variables $B$ and $G$, $q(B,G) = q(B)q(G)$, so:

$$\begin{aligned} log(p(D_{train})) \geq &\sum_B \int_G \log(p(D_{train}|B,G))q(B)q_V(G)dG \\ &- KL(q(B)||p(B)) - KL(q_V(G)||p(G)) \end{aligned} \tag{14}$$

For a spike-and-slab distribution, each element of $G$ is independently sampled from a Gaussian distribution, $\mathcal{N}(v_{i,j}, \sigma^2_{v_{i,j}})$, where $\sigma^2_{v_{i,j}} = \alpha\mu^2_{v_{i,j}}$. $G$ can be sampled using the Gaussian "reparameterization trick". This allows Equation 14 to be rewritten as:

$$\begin{aligned}\log(p(D_{train})) \geq \sum_B \int_\epsilon & \log(p(D_{train}|B, G)q(\epsilon)q(B)d\epsilon \\ & - KL(q(B)||p(B)) - KL(q_V(G)||p(G))\end{aligned} \tag{15}$$

$\epsilon$ is a vector containing each $\epsilon_{i,j}$.

This results in the following minimization objective function:

$$\mathcal{L}_V := -\sum_B \int_\epsilon \log(p(D_{train}|B, G))q(\epsilon)q(B)d\epsilon + KL(q(B)||p(B)) + KL(q_V(G)||p(G) \tag{16}$$

Using $Bern(1 - p_{do})$ as a prior for each element of $B$ leads to a constant KLD of zero for Bernoulli dropout with a drop probability of $p_{do}$ and using a prior of $\mathcal{N}(0, \sigma^2_p)$ for each element of $G$ leads to L2-regularization being a lowerbound of the KLD between $q_V(G)$ and $\mathcal{N}(0, \lambda^{-1})$:

$$\mathcal{L}_V \geq \widetilde{\mathcal{L}}_V := -\sum_B \int_\epsilon \log(p(D_{train}|B, G))q(\epsilon)q(B)d\epsilon + \frac{\lambda}{2}\mathbf{v}\mathbf{v}^\intercal \tag{17}$$

where $\mathbf{v}$ is a vector containing each $v_{i,j}$ and $\epsilon$ is a vector containing each $\epsilon_{i,j}$.

Approximating using Monte Carlo integration for training (Eq. 18) and testing (Eq. 19):

$$\widetilde{\mathcal{L}}_V :\approx -\frac{1}{n}\sum_{(B,\epsilon)} \log(p(D_{train}|B, G)) + \frac{\lambda}{2}\mathbf{v}\mathbf{v}^\intercal \tag{18}$$

$$p(D_{test}) \approx \frac{1}{n}\sum_{(B,\epsilon)} p(D_{test}|B, G) \tag{19}$$

where $b_{i,*} \sim Bern(1 - p_{do})$ and $\epsilon_{i,j} \sim \mathcal{N}(0, 1)$.

# 2 Experiments

## 2.1 Architectures

Table 1: The convolutional neural network (CNN) architecture used for MNIST.

| Layer | Kernel Size | # Features | Stride | Non-linearity |
|---|---|---|---|---|
| Conv-1 | 5x5 | 32 | 1 | ReLU |
| MaxPool-1 | 2x2 | 32 | 2 | Max |
| Conv-2 | 5x5 | 64 | 1 | ReLU |
| MaxPool-2 | 2x2 | 64 | 2 | Max |
| FC | 1500 | 500 | - | ReLU |
| FC | 500 | 10 | - | Softmax |

Table 2: The convolutional neural network (CNN) architecture used for CIFAR-10.

| Layer | Kernel Size | # Features | Stride | Non-linearity |
|---|---|---|---|---|
| Conv-1 | 3x3 | 64 | 1 | ReLU |
| Conv-2 | 3x3 | 64 | 1 | ReLU |
| MaxPool-1 | 2x2 | 64 | 2 | Max |
| Conv-3 | 3x3 | 128 | 1 | ReLU |
| Conv-4 | 3x3 | 128 | 1 | ReLU |
| MaxPool-2 | 2x2 | 128 | 2 | Max |
| Conv-5 | 3x3 | 256 | 1 | ReLU |
| Conv-6 | 3x3 | 256 | 1 | ReLU |
| Conv-7 | 3x3 | 256 | 1 | ReLU |
| MaxPool-3 | 2x2 | 256 | 2 | Max |
| Conv-8 | 3x3 | 512 | 1 | ReLU |
| Conv-9 | 3x3 | 512 | 1 | ReLU |
| Conv-10 | 3x3 | 512 | 1 | ReLU |
| MaxPool-4 | 2x2 | 512 | 2 | Max |
| Conv-11 | 3x3 | 512 | 1 | ReLU |
| Conv-12 | 3x3 | 512 | 1 | ReLU |
| Conv-13 | 3x3 | 512 | 1 | ReLU |
| MaxPool-5 | 2x2 | 512 | 2 | Max |
| FC | 512 | 512 | - | ReLU |
| FC | 512 | 10 | - | Softmax |

## 2.2 Additional results

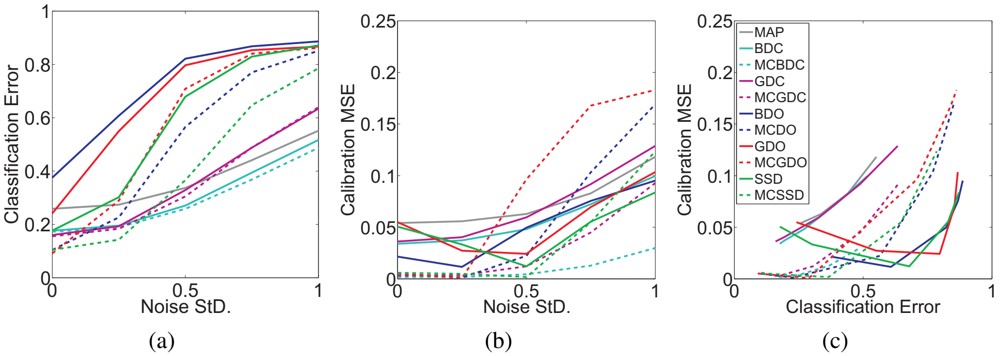


Figure 1: The CIFAR-10 (a) classification error for additive Gaussian noise using standard deviations St.D of 0, 0.25, 0.5, 0.75, and 1, (b) mean squared error (MSE) between the $x = y$ line and the calibration plot (i.e. the frequency of the true label vs predicted probability of that label) for varying Gaussian image noise StD., and (c) calibration MSE versus the classification error for predicitons across all noise StD. for Bernoulli dropconnect (BDC), Gaussian dropconnect (GDC), Bernoulli dropout (BDO), Gaussian dropout (GDO), and spike-and-slab dropout (SSD) with and without MC sampling using 10 samples. For all dropconnect and dropout methods, $p = 0.5$. For spike-and-slab, $p_{do} = 0.5$ and $p_{dc} = 0.1$.

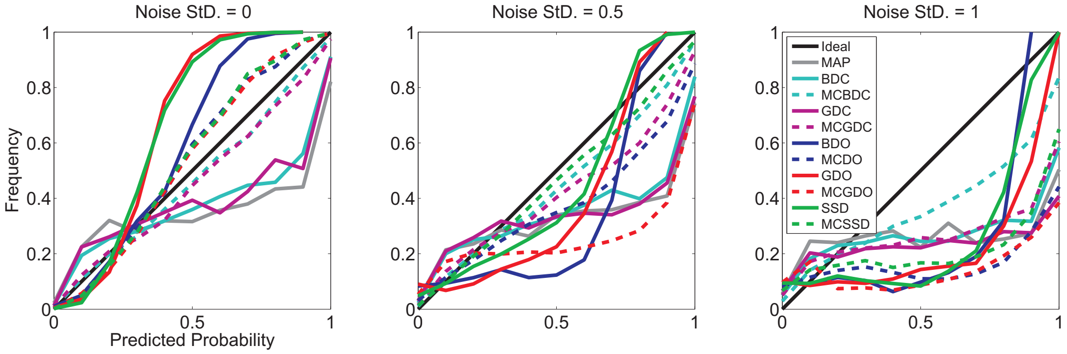


Figure 2: The $x = y$ line (Ideal) and the calibration plot (i.e. the frequency of the true label vs predicted probability of that label) for varying Gaussian image noise StD. for the CIFAR-10 trained Bernoulli dropconnect (BDC), Gaussian dropconnect (GDC), Bernoulli dropout (BDO), Gaussian dropout (GDO), and spike-and-slab dropout (SSD) networks with and without MC sampling using 10 samples. For all dropconnect and dropout methods, $p = 0.5$. For spike-and-slab, $p_{do} = 0.5$ and $p_{dc} = 0.1$.

## References


[1] David Barber and Christopher M Bishop. Ensemble learning in bayesian neural networks. *NATO ASI SERIES F COMPUTER AND SYSTEMS SCIENCES*, 168:215–238, 1998.

[2] Charles Blundell, Julien Cornebise, Koray Kavukcuoglu, and Daan Wierstra. Weight uncertainty in neural network. In *Proceedings of The 32nd International Conference on Machine Learning*, pages 1613–1622, 2015.

[3] Alex Graves. Practical variational inference for neural networks. In *Advances in Neural Information Processing Systems*, pages 2348–2356, 2011.

[4] Geoffrey E Hinton and Drew Van Camp. Keeping the neural networks simple by minimizing the description length of the weights. In *Proceedings of the sixth annual conference on Computational learning theory*, pages 5–13. ACM, 1993.

[5] Diederik P Kingma, Tim Salimans, and Max Welling. Variational dropout and the local reparameterization trick. In *Advances in Neural Information Processing Systems*, pages 2575–2583, 2015.

[6] Michalis K Titsias and Miguel Lázaro-Gredilla. Spike and slab variational inference for multi-task and multiple kernel learning. In *Advances in neural information processing systems*, pages 2339–2347, 2011.
